# Supplementary material for: Feature Embedding by Template Matching as a ResNet Block
Source: arXiv:2210.00992 source file (2023-08-15)
Supplement: Supplementary file 1 [file fig_template.tex]

% Below is an example of how to insert images. Delete the ``\vspace'' line,
% uncomment the preceding line ``\centerline...'' and replace ``imageX.ps''
% with a suitable PostScript file name.
% -------------------------------------------------------------------------
\begin{figure}[htb]

\begin{minipage}[b]{1.0\linewidth}
  \centering
  \centerline{\includegraphics[width=8.5cm]{figures/image1.png}}
%  \vspace{2.0cm}
  \centerline{(a) Result 1}\medskip
\end{minipage}
%
\begin{minipage}[b]{.48\linewidth}
  \centering
  \centerline{\includegraphics[width=4.0cm]{figures/image3.png}}
%  \vspace{1.5cm}
  \centerline{(b) Results 3}\medskip
\end{minipage}
\hfill
\begin{minipage}[b]{0.48\linewidth}
  \centering
  \centerline{\includegraphics[width=4.0cm]{figures/image4.png}}
%  \vspace{1.5cm}
  \centerline{(c) Result 4}\medskip
\end{minipage}
%
\caption{Example of placing a figure with experimental results.}
\label{fig:res}
%
\end{figure}
